# Supplementary material for: NeRD: Neural Reflectance Decomposition from Image Collections
Source: arXiv:2012.03918 source file (2021-08-26)
Supplement: Supplementary file 1 [file comparison_old.tex]

\normalsize%
\renewcommand{\arraystretch}{0.6}%
\setlength{\tabcolsep}{0pt}%
\begin{tabular}{@{}l>{\centering\arraybackslash}m{50pt}>{\centering\arraybackslash}m{50pt}>{\centering\arraybackslash}m{50pt}>{\centering\arraybackslash}m{50pt}>{\centering\arraybackslash}m{100pt}>{\centering\arraybackslash}m{50pt}>{\centering\arraybackslash}m{50pt}>{\centering\arraybackslash}m{50pt}@{}}%
\toprule%
&\footnotesize Base Color&\footnotesize Metalness&\footnotesize Roughness&\footnotesize Normal&\footnotesize Environment&\footnotesize Image&\footnotesize Novel 1& \footnotesize Novel 2\\%
\midrule%
\rotatebox[origin=c]{90}{\footnotesize Ours}&\includegraphics[width=50pt]{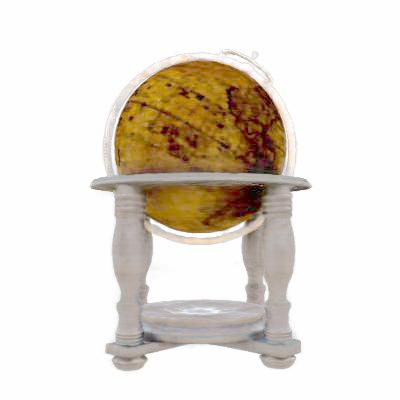}&\includegraphics[width=50pt]{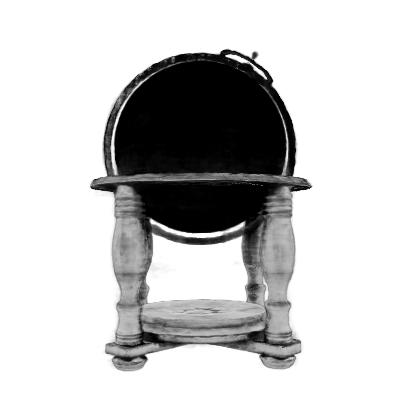}&\includegraphics[width=50pt]{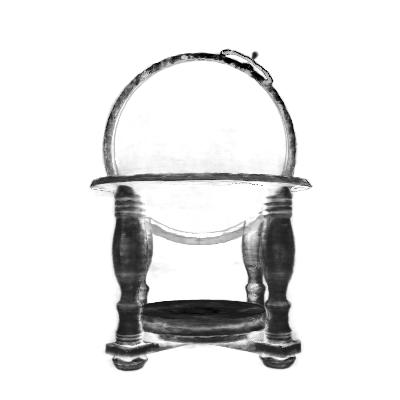}&\includegraphics[width=50pt]{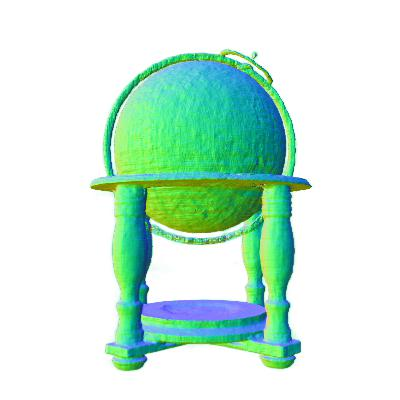}&\includegraphics[width=100pt]{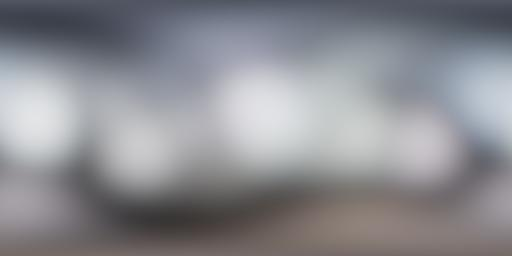}&\includegraphics[width=50pt]{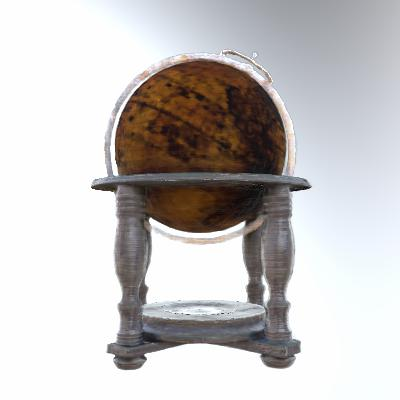}&\includegraphics[width=50pt]{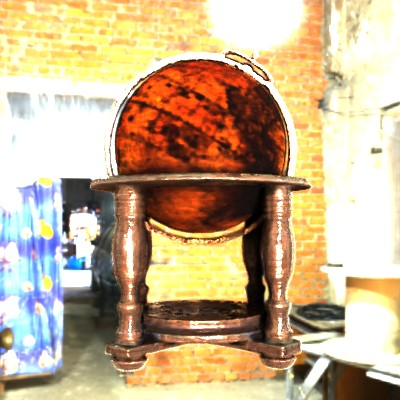}&\includegraphics[width=50pt]{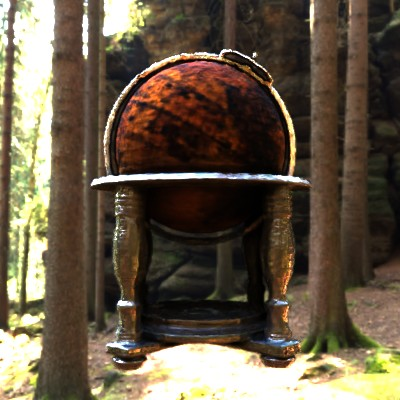}\\%
%
\scriptsize MSE&\scriptsize0.0739&\scriptsize 0.0735&\scriptsize 0.2702&\scriptsize 0.0086&\scriptsize 0.0456&\scriptsize 0.0140&\scriptsize 0.0884&\scriptsize 0.0654\\%
%All&0.0361&0.0408&0.1650&0.0116&0.0830&0.0229\\%
\rotatebox[origin=c]{90}{\footnotesize GT}&\includegraphics[width=50pt]{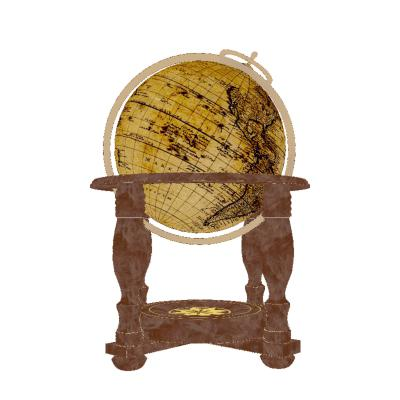}&\includegraphics[width=50pt]{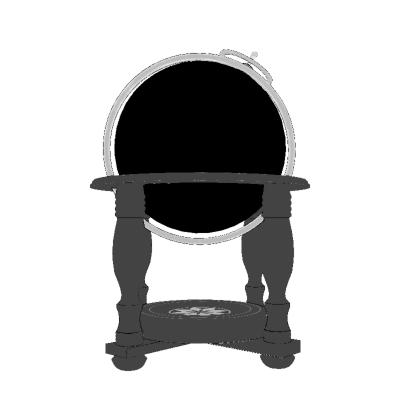}&\includegraphics[width=50pt]{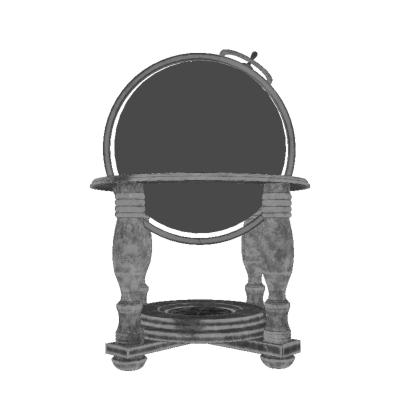}&\includegraphics[width=50pt]{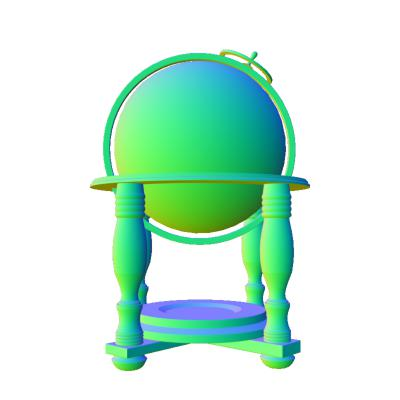}&\includegraphics[width=100pt]{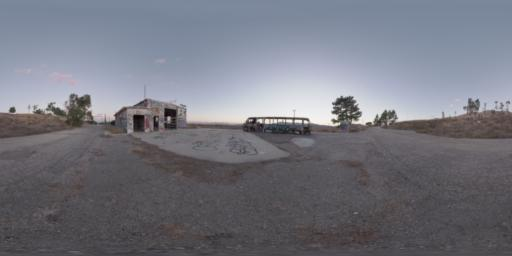}&\includegraphics[width=50pt]{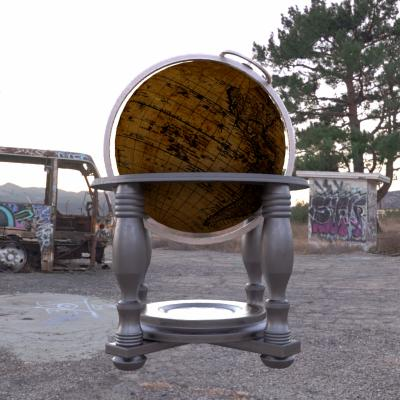}&\includegraphics[width=50pt]{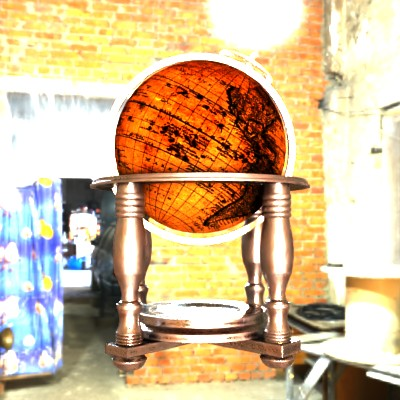}&\includegraphics[width=50pt]{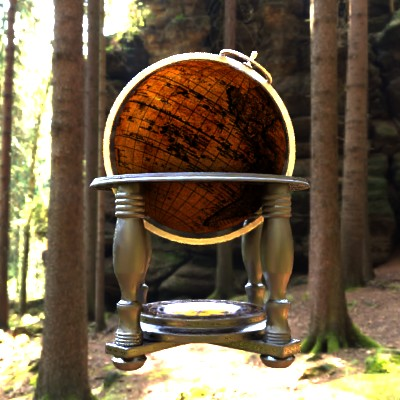}\\\bottomrule%
\end{tabular}\\[1.5ex]
%
\begin{tabular}{@{}%
>{\centering\arraybackslash}m{50pt}>{\centering\arraybackslash}m{50pt}@{\hskip 1mm}l@{\hskip 1.5mm}%
>{\centering\arraybackslash}m{50pt}>{\centering\arraybackslash}m{50pt}@{\hskip 1mm}l@{\hskip 1.5mm}%
>{\centering\arraybackslash}m{50pt}>{\centering\arraybackslash}m{50pt}@{\hskip 1mm}l@{\hskip 1.5mm}%
>{\centering\arraybackslash}m{50pt}>{\centering\arraybackslash}m{50pt}@{\hskip 1mm}l@{}}%
\includegraphics[width=50pt]{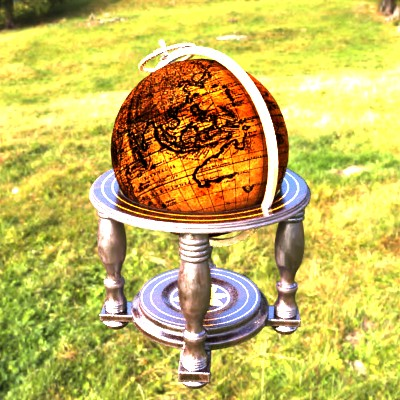}&\includegraphics[width=50pt]{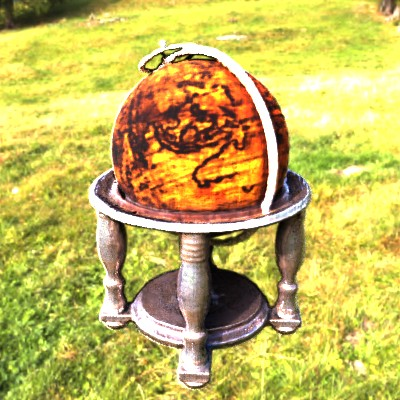}&\rotatebox[origin=c]{90}{\scriptsize MSE: 0.0750}&
\includegraphics[width=50pt]{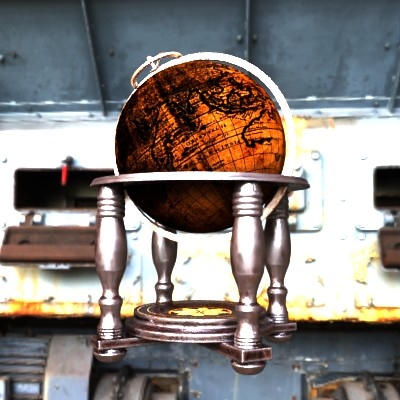}&\includegraphics[width=50pt]{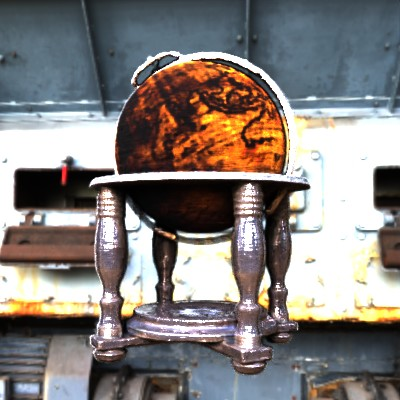}&\rotatebox[origin=c]{90}{\scriptsize MSE: 0.0515}&
\includegraphics[width=50pt]{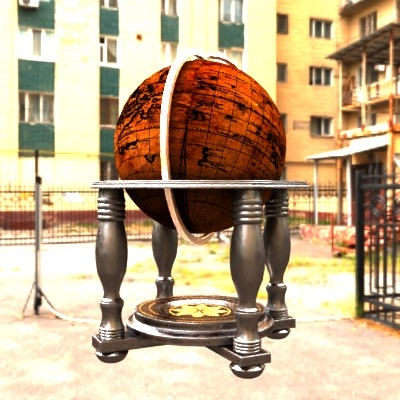}&\includegraphics[width=50pt]{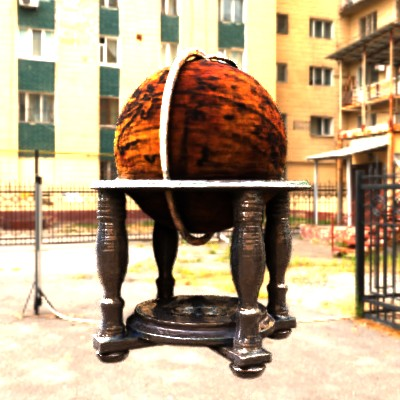}&\rotatebox[origin=c]{90}{\scriptsize MSE: 0.0454}&
\includegraphics[width=50pt]{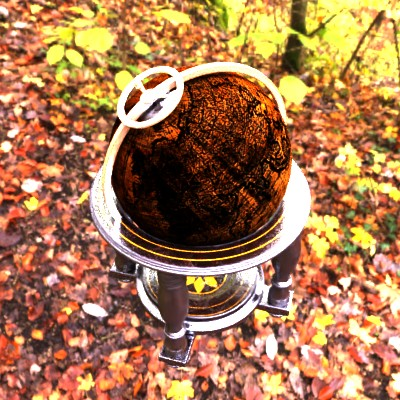}&\includegraphics[width=50pt]{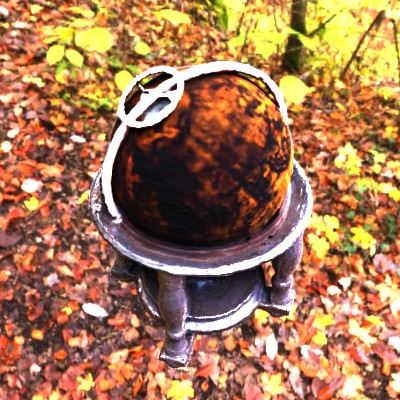}&\rotatebox[origin=c]{90}{\scriptsize MSE: 0.0571}\\%
\footnotesize GT&\footnotesize Ours&&\footnotesize GT&\footnotesize Ours&&\footnotesize GT&\footnotesize Ours&&\footnotesize GT&\footnotesize Ours \\\bottomrule%
\end{tabular}
